# Supplementary material for: Stable nanofacets in [111] tilt grain boundaries of face-centered cubic metals
Source: arXiv:2309.07595 ancillary file (2024-04-22)
Supplement: Supplementary file 1 [file supplemental.pdf]

# SUPPLEMENTAL MATERIAL
# Stable nanofacets in [111] tilt grain boundaries of face-centered cubic metals

Tobias Brink, Lena Langenohl, Swetha Pemma, Christian H. Liebscher, and Gerhard Dehm
*Max-Planck-Institut für Eisenforschung GmbH, Max-Planck-Straße 1, 40237 Düsseldorf, Germany*

## I. ATOMIC STRUCTURE

### A. $\Sigma19b$ ($\theta = 46.83°$)

Σ19b, domino

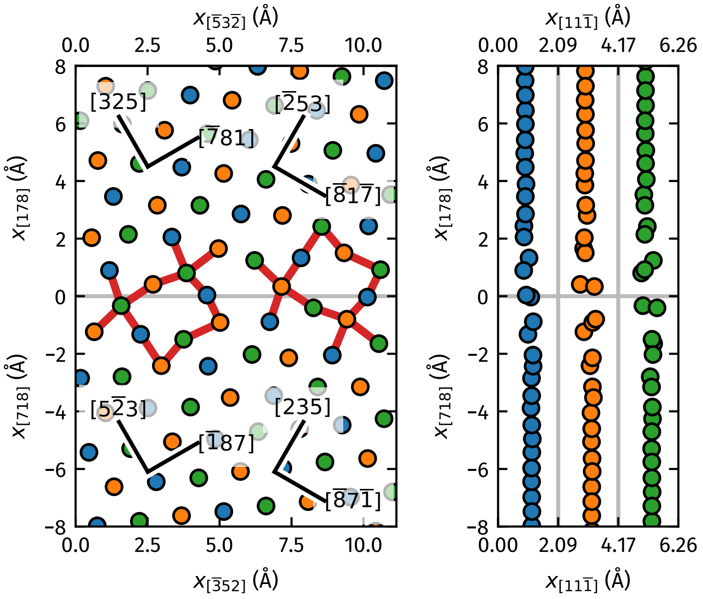


**Supplemental Fig. S1:** Domino motif in a $\Sigma19b$ $[11\bar{1}]$ $\{178\}$ symmetric tilt GB. One unit cell is shown.

(a) Σ19b, left zipper

(b) Σ19b, right zipper

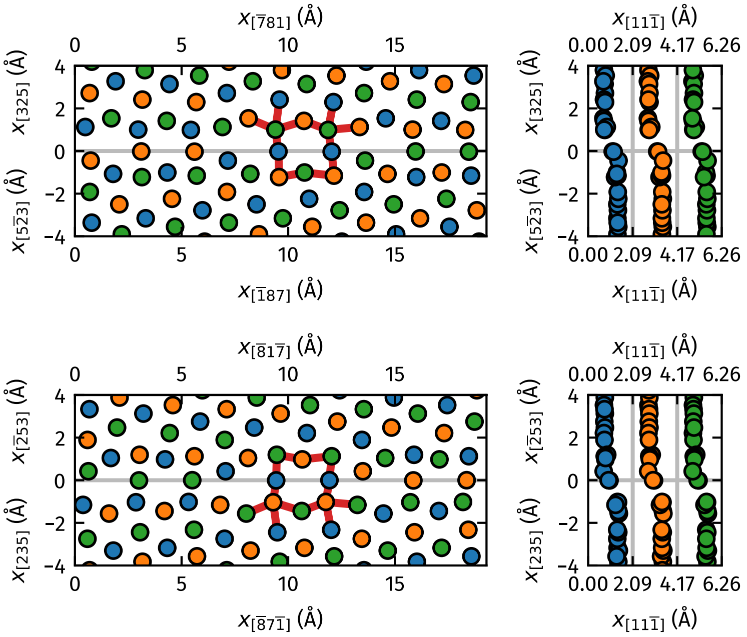


**Supplemental Fig. S2:** Zipper motifs in $\Sigma19b$ $[11\bar{1}]$ $\{235\}$ symmetric tilt GBs. The motifs are labeled left (a) and right (b) according to how they also occur in Fig. S1. One unit cell is shown.

(a) Σ19b, left zipper overlayed over domino

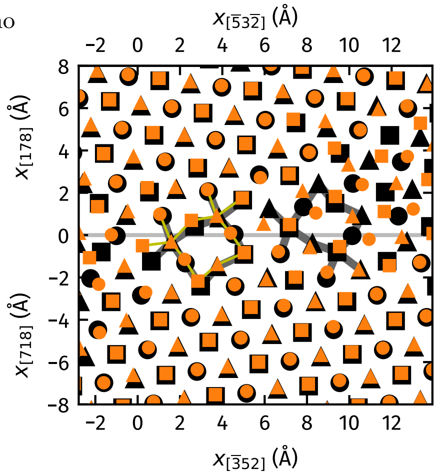


(b) Σ19b, right zipper overlayed over domino

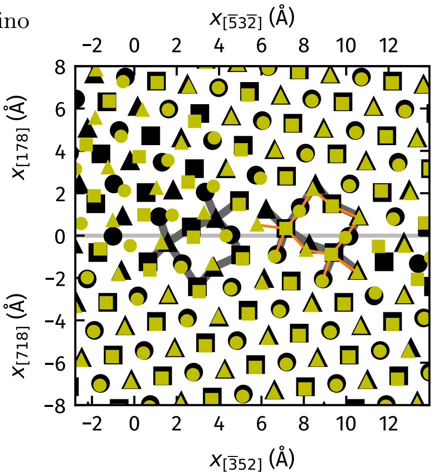


(c) Σ19b, both zippers overlayed over domino

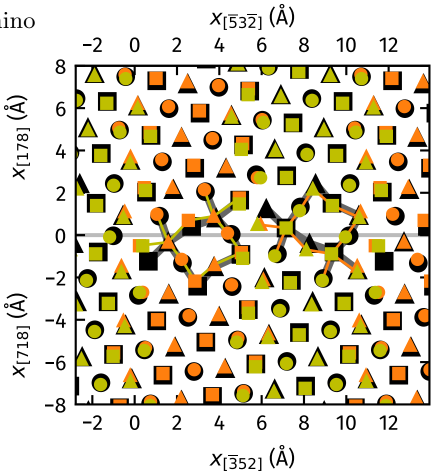


**Supplemental Fig. S3:** Illustration of overlaying the left and right zipper structures over the domino structure in the Σ19b tilt GB. First, a single zipper structure is rotated by +30° (a, left zipper) or −30° (b, right zipper) and plotted over the domino motif. Orange and yellow atoms belong to the left and right zipper, respectively, while black atoms belong to the domino structure. In the regions where each zipper is overlayed over its respective facet of the domino structure, the fit is perfect. (c) If using each zipper only in the region where it fits, the overlap is perfect everywhere. Different symbol shapes indicate A/B/C stacking.

## B. Σ37c ($\theta = 50.57°$)

Σ37c, domino

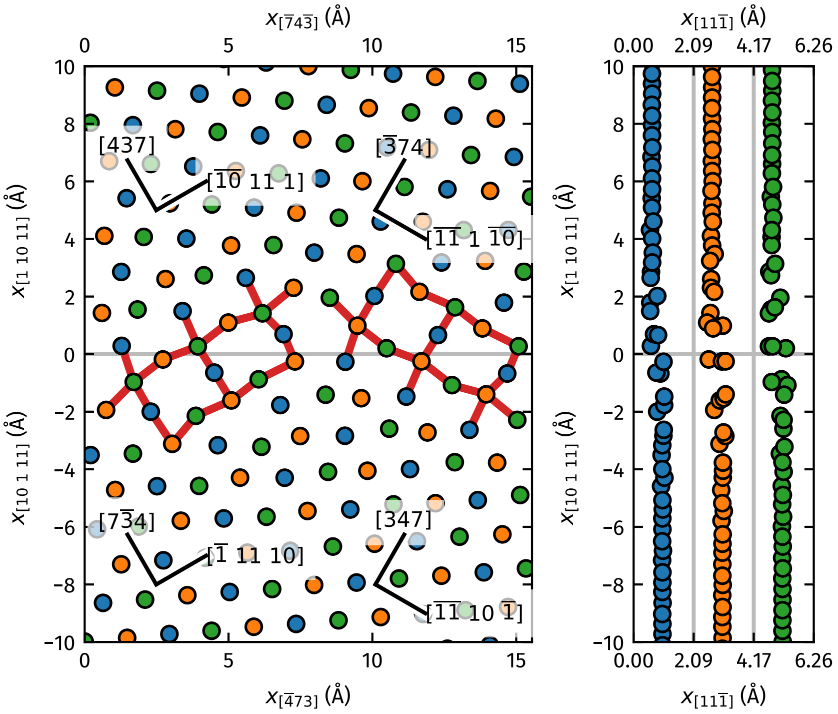


**Supplemental Fig. S4:** Domino motif in a Σ37c $[11\bar{1}]$ $\{1\,10\,11\}$ symmetric tilt GB. One unit cell is shown.

(a) Σ37c, left zipper

(b) Σ37c, right zipper

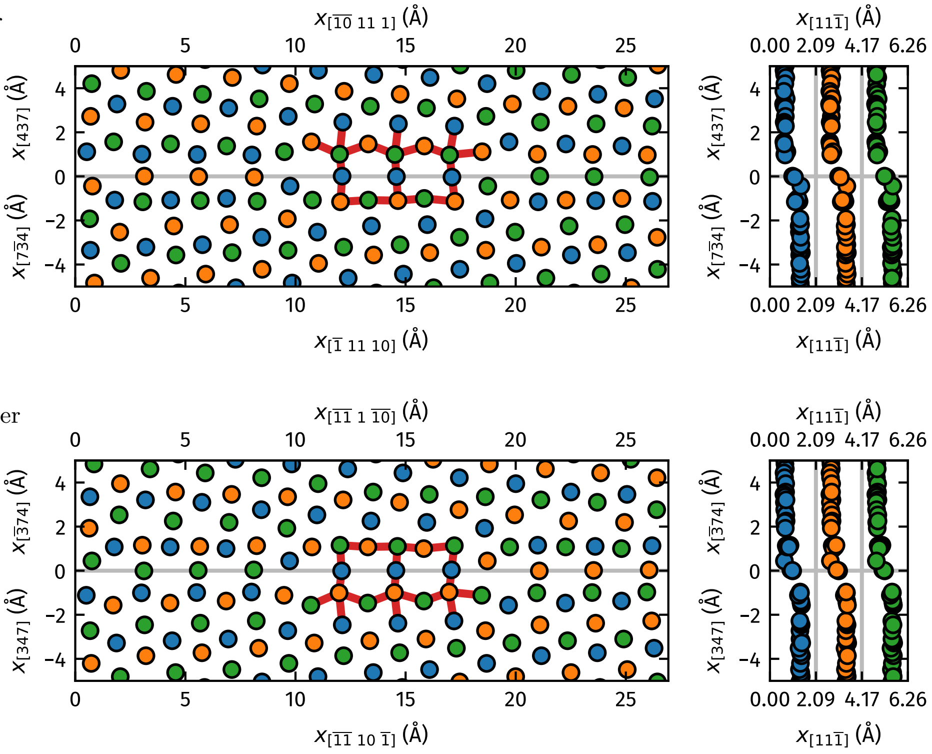


**Supplemental Fig. S5:** Zipper motifs in Σ37c $[11\bar{1}]$ $\{347\}$ symmetric tilt GBs. The motifs are labeled left (a) and right (b) according to how they also occur in Fig. S4. One unit cell is shown.

(a) Σ37c, left zipper overlayed over domino

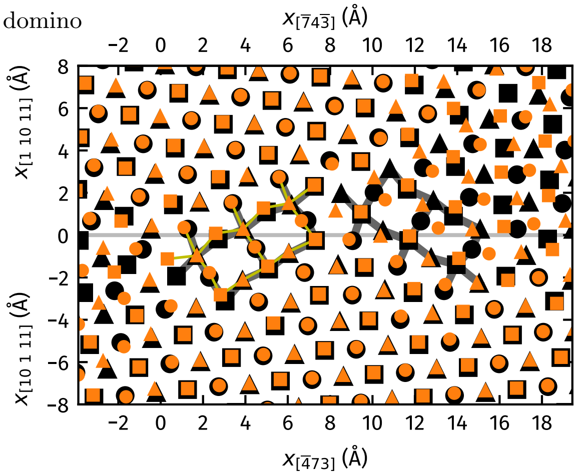


(b) Σ37c, right zipper overlayed over domino

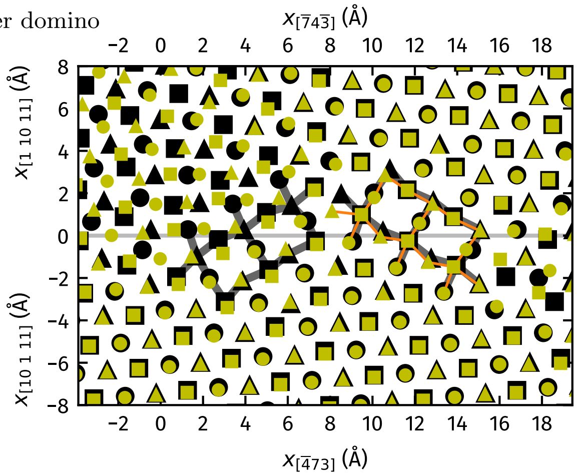


(c) Σ37c, both zippers overlayed over domino

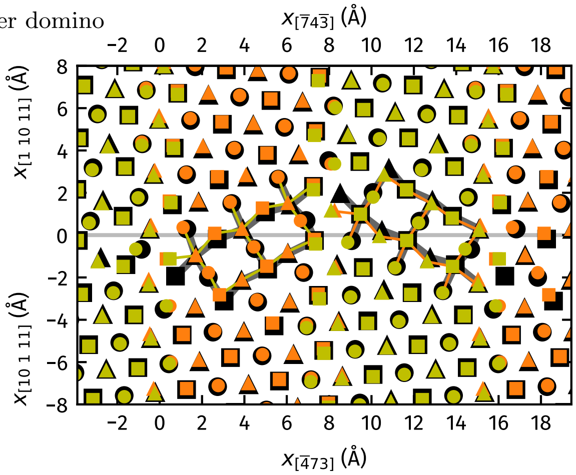


**Supplemental Fig. S6:** Illustration of overlaying the left and right zipper structures over the domino structure in the Σ37c tilt GB. First, a single zipper structure is rotated by +30° (a, left zipper) or −30° (b, right zipper) and plotted over the domino motif. Orange and yellow atoms belong to the left and right zipper, respectively, while black atoms belong to the domino structure. In the regions where each zipper is overlayed over its respective facet of the domino structure, the fit is perfect. (c) If using each zipper only in the region where it fits, the overlap is perfect everywhere. Different symbol shapes indicate A/B/C stacking.

### C. $\Sigma 61b$ ($\theta = 53.66°$)

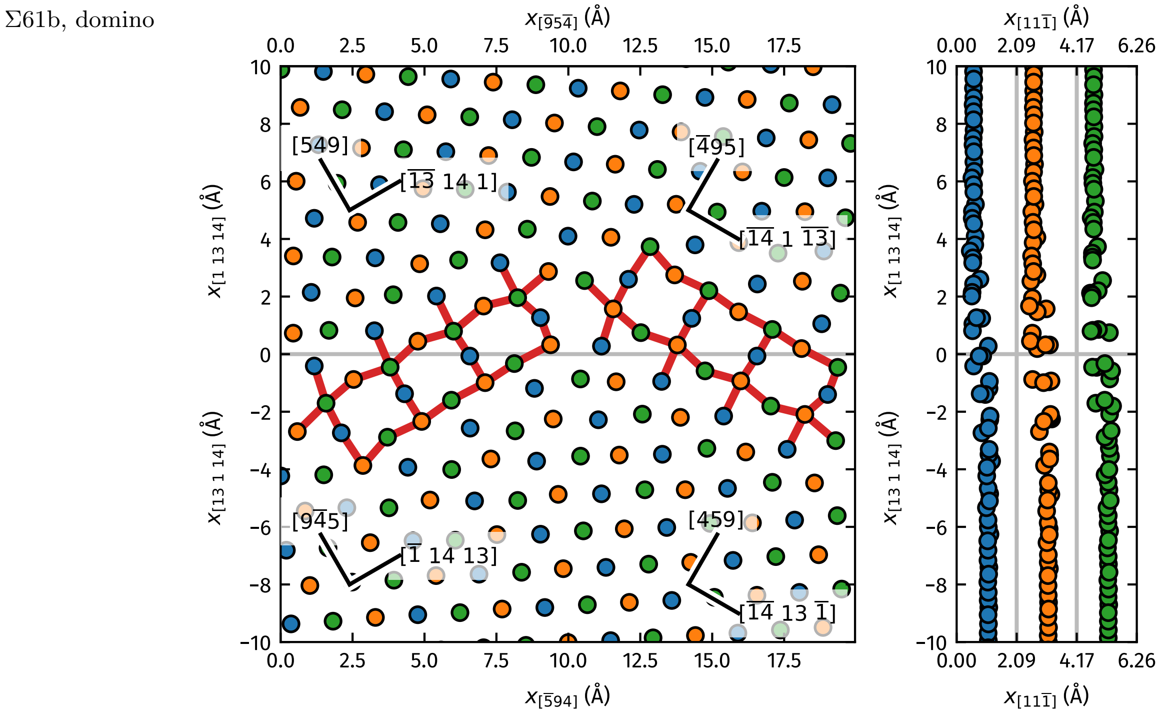


**Supplemental Fig. S7:** Domino motif in a $\Sigma 61b$ $[11\bar{1}]$ $\{1\,13\,14\}$ symmetric tilt GB. One unit cell is shown.

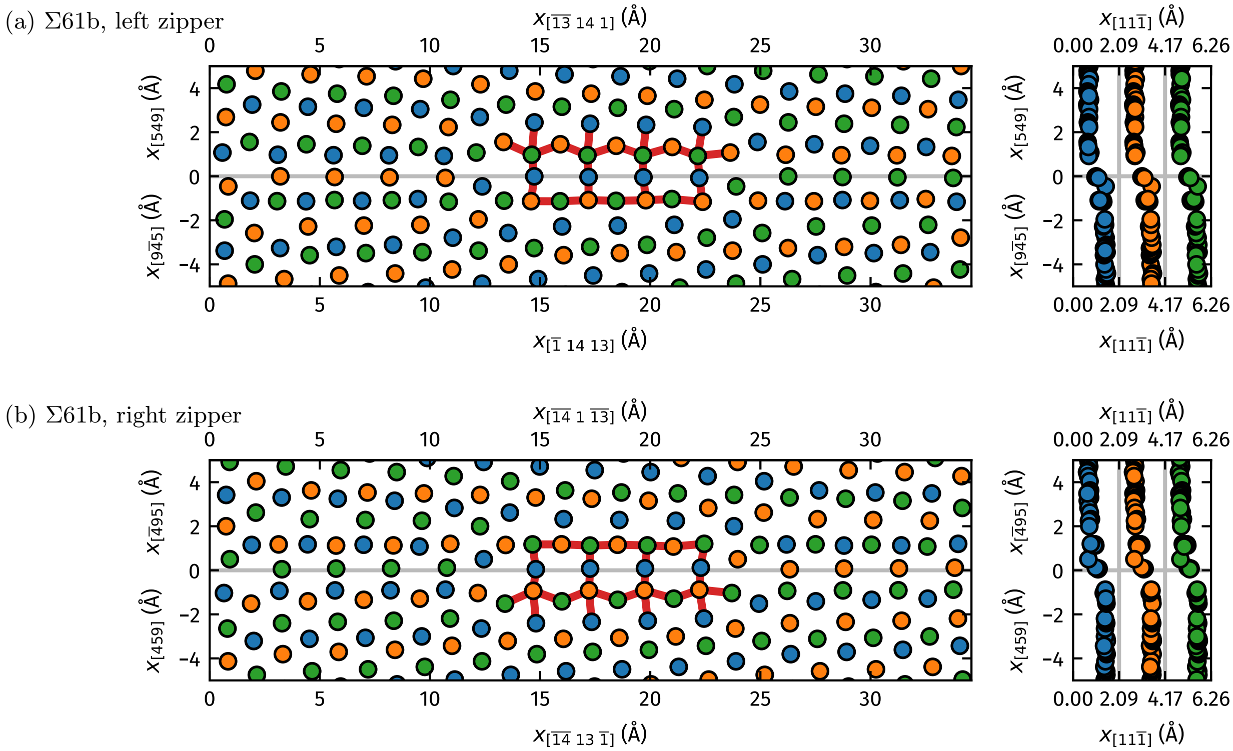


**Supplemental Fig. S8:** Zipper motifs in $\Sigma 61b$ $[11\bar{1}]$ $\{459\}$ symmetric tilt GBs. The motifs are labeled left (a) and right (b) according to how they also occur in Fig. S7. One unit cell is shown.

(a) Σ61b, left zipper overlayed over domino

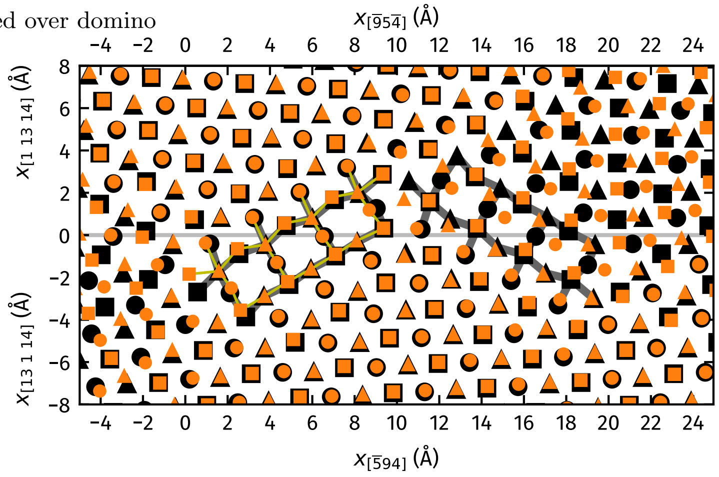


(b) Σ61b, right zipper overlayed over domino

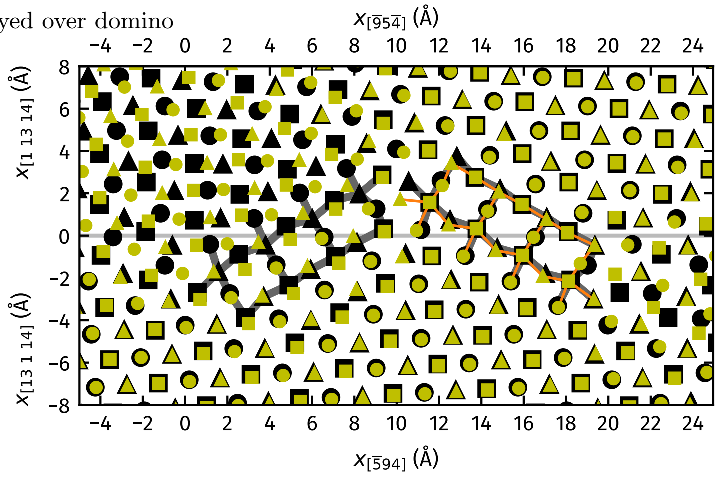


(c) Σ61b, both zippers overlayed over domino

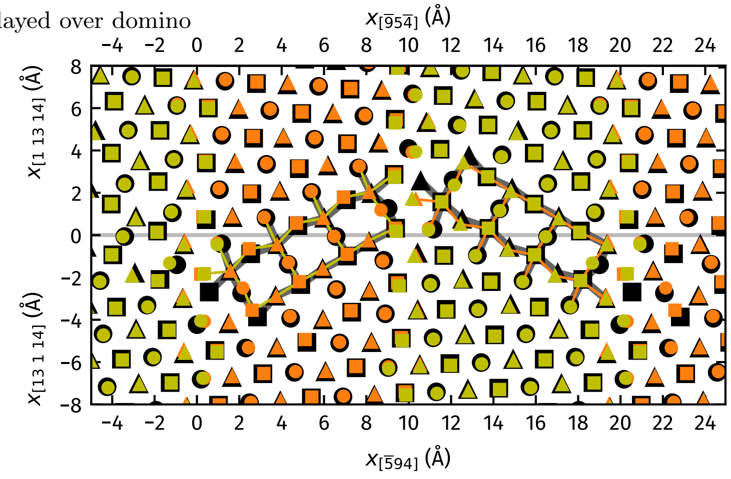


**Supplemental Fig. S9:** Illustration of overlaying the left and right zipper structures over the domino structure in the Σ61b tilt GB. First, a single zipper structure is rotated by +30° (a, left zipper) or −30° (b, right zipper) and plotted over the domino motif. Orange and yellow atoms belong to the left and right zipper, respectively, while black atoms belong to the domino structure. In the regions where each zipper is overlayed over its respective facet of the domino structure, the fit is perfect. (c) If using each zipper only in the region where it fits, the overlap is perfect everywhere. Different symbol shapes indicate A/B/C stacking.

### D. $\Sigma 127$ ($\theta = 54.91°$)

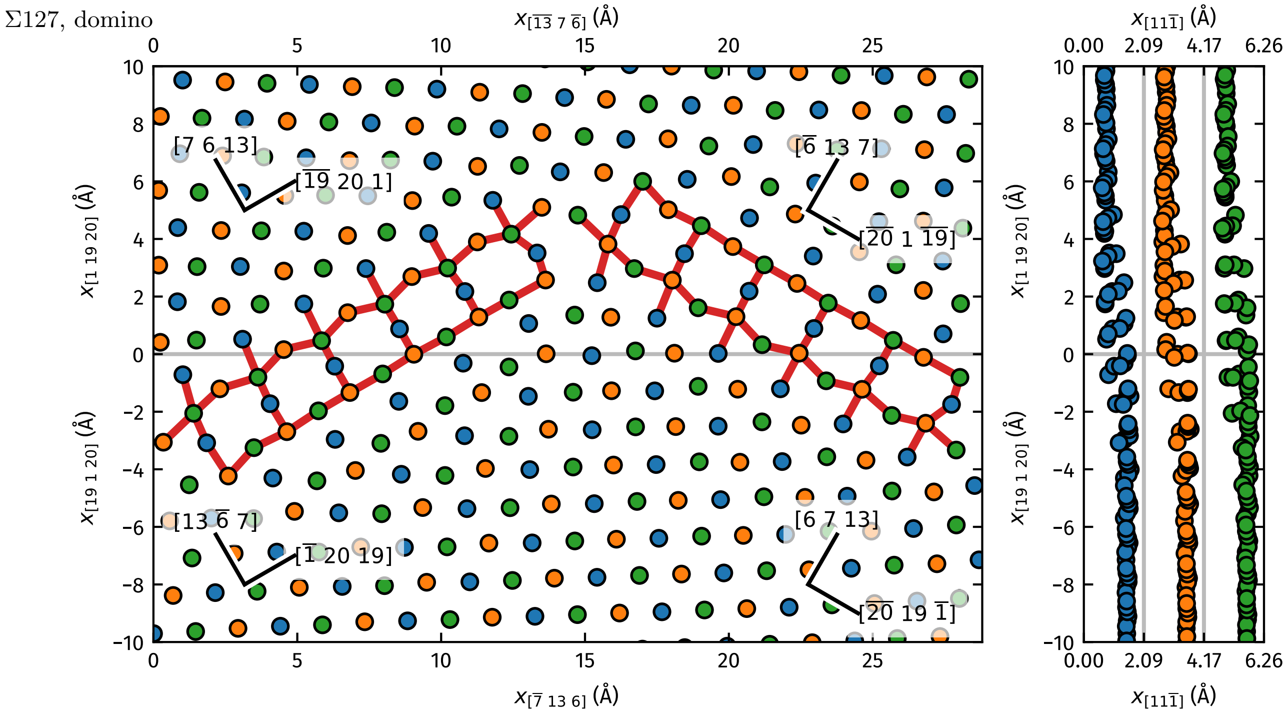


**Supplemental Fig. S10:** Domino motif in a $\Sigma 127$ $[11\bar{1}]$ $\{1\,19\,20\}$ symmetric tilt GB. One unit cell is shown.

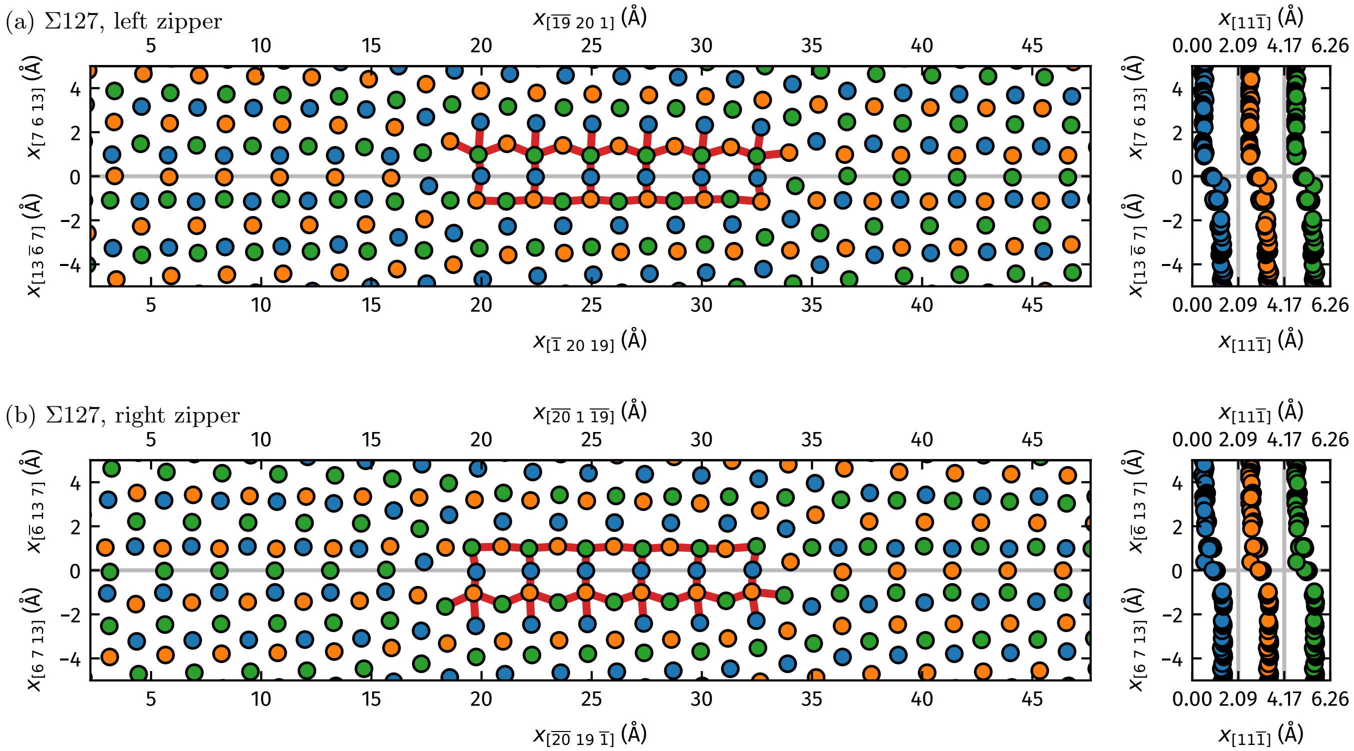


**Supplemental Fig. S11:** Zipper motifs in $\Sigma 127$ $[11\bar{1}]$ $\{6\,7\,13\}$ symmetric tilt GBs. The motifs are labeled left (a) and right (b) according to how they also occur in Fig. S10. Unit cells are only shown partially due to their large size.

(a) Σ127, left zipper overlayed over domino

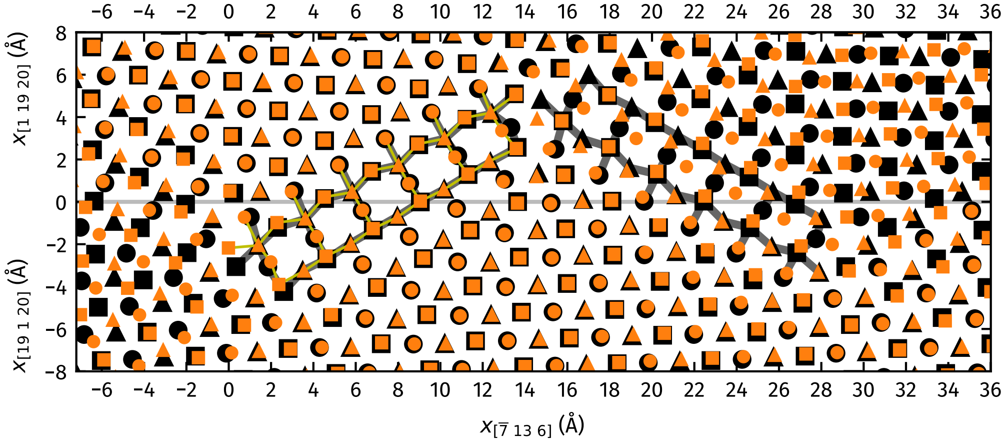


(b) Σ127, right zipper overlayed over domino

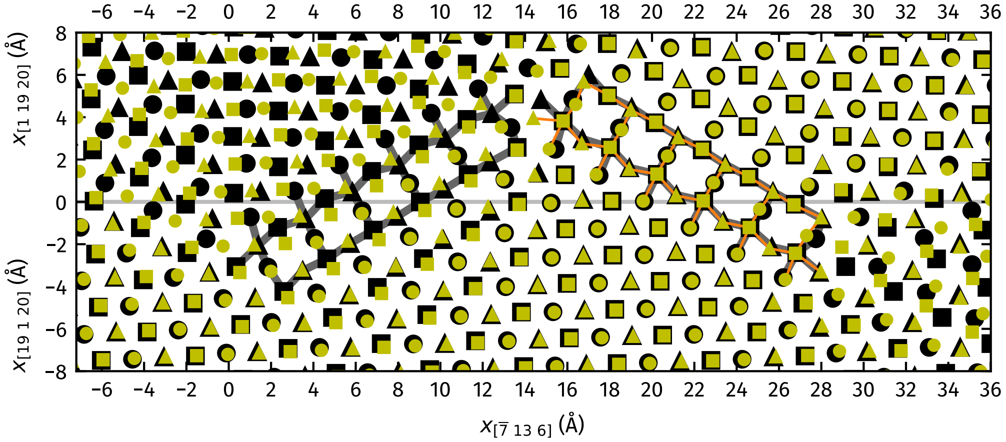


(c) Σ127, both zippers overlayed over domino

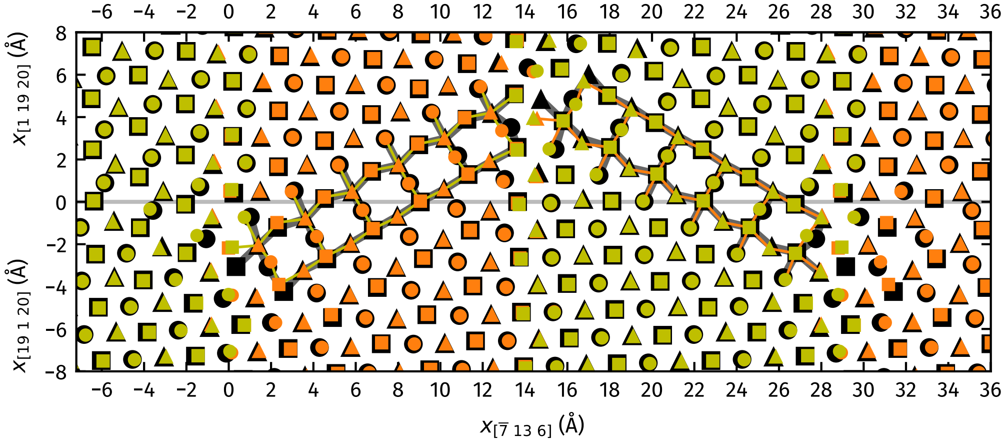


**Supplemental Fig. S12:** Illustration of overlaying the left and right zipper structures over the domino structure in the Σ127 tilt GB. First, a single zipper structure is rotated by $+30°$ (a, left zipper) or $-30°$ (b, right zipper) and plotted over the domino motif. Orange and yellow atoms belong to the left and right zipper, respectively, while black atoms belong to the domino structure. In the regions where each zipper is overlayed over its respective facet of the domino structure, the fit is perfect. (c) If using each zipper only in the region where it fits, the overlap is perfect everywhere. Different symbol shapes indicate A/B/C stacking.

### E. Σ169b ($\theta = 55.59°$)

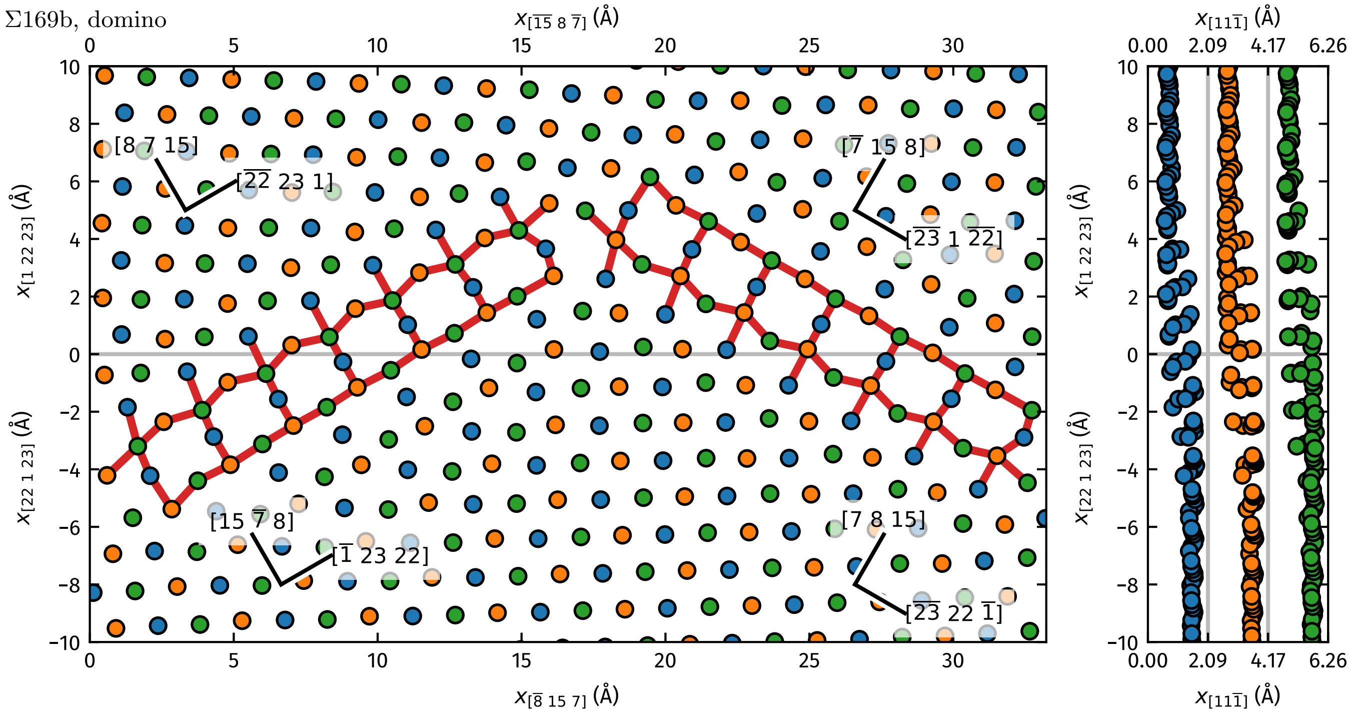


**Supplemental Fig. S13:** Domino motif in a Σ169b $[11\bar{1}]$ $\{1\,22\,23\}$ symmetric tilt GB. One unit cell is shown.

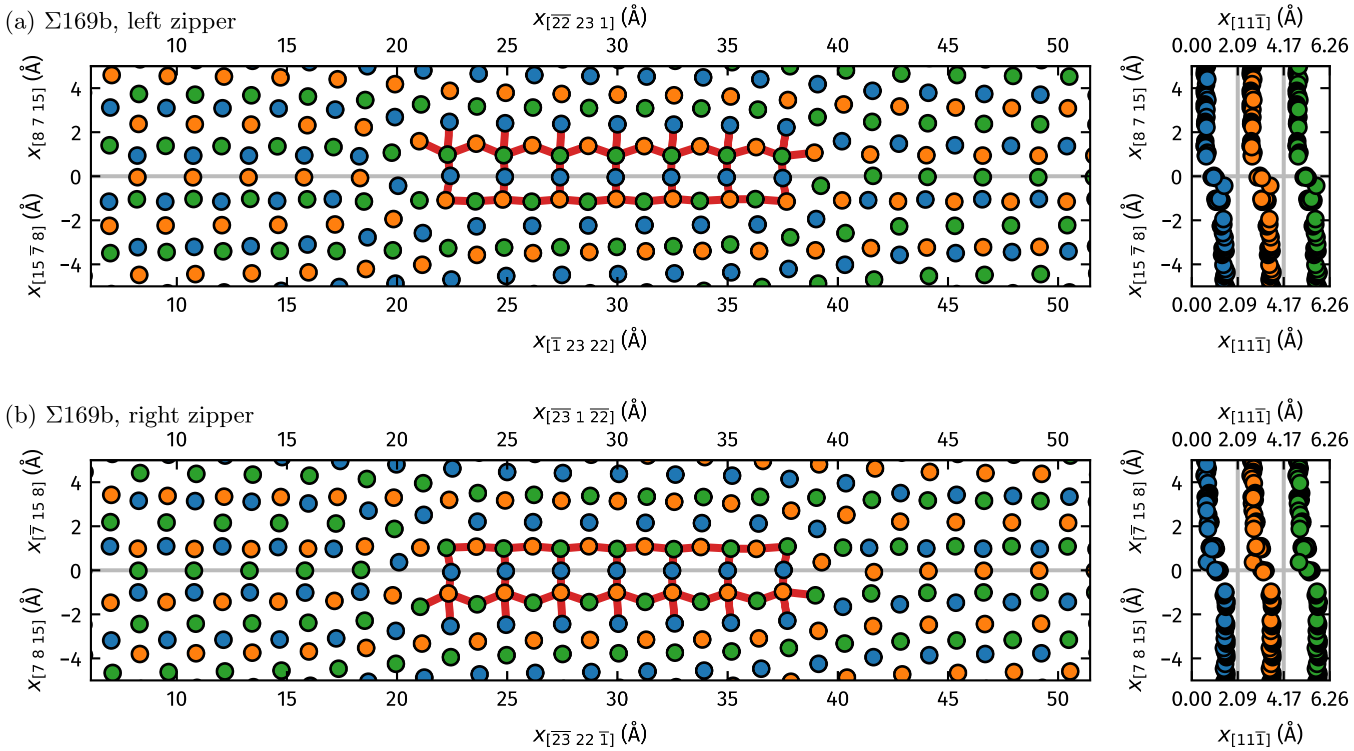


**Supplemental Fig. S14:** Zipper motifs in Σ169b $[11\bar{1}]$ $\{7\,8\,15\}$ symmetric tilt GBs. The motifs are labeled left (a) and right (b) according to how they also occur in Fig. S13. Unit cells are only shown partially due to their large size.

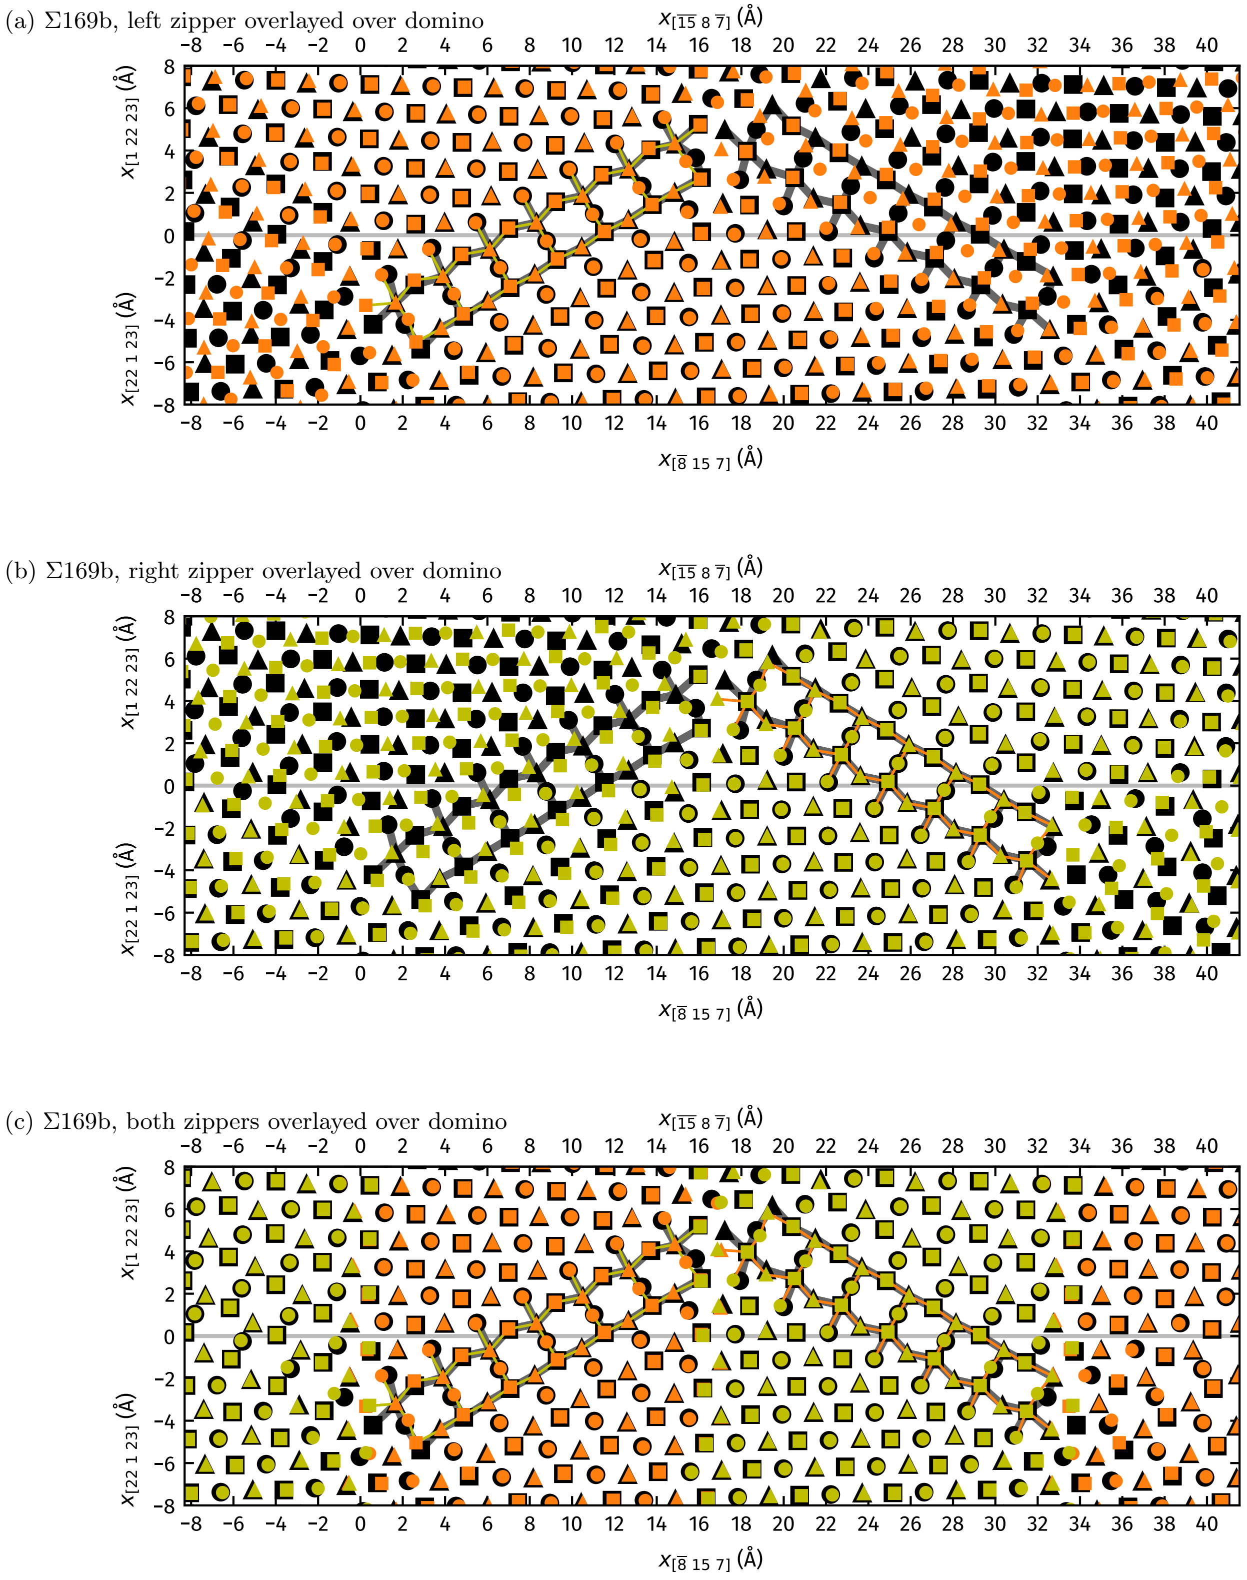


**Supplemental Fig. S15:** Illustration of overlaying the left and right zipper structures over the domino structure in the Σ169b tilt GB. First, a single zipper structure is rotated by +30° (a, left zipper) or −30° (b, right zipper) and plotted over the domino motif. Orange and yellow atoms belong to the left and right zipper, respectively, while black atoms belong to the domino structure. In the regions where each zipper is overlayed over its respective facet of the domino structure, the fit is perfect. (c) If using each zipper only in the region where it fits, the overlap is perfect everywhere. Different symbol shapes indicate A/B/C stacking.

## F. $\Sigma 3$ ($\theta = 60°$)

(a) Σ3, left zipper

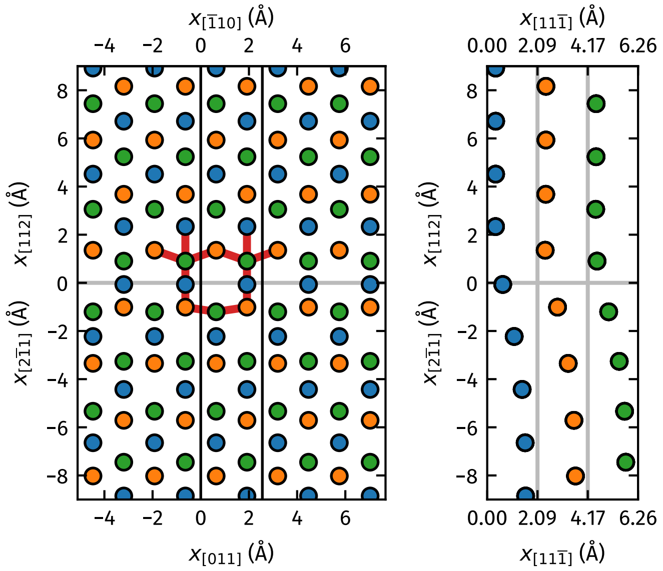


(b) Σ3, right zipper

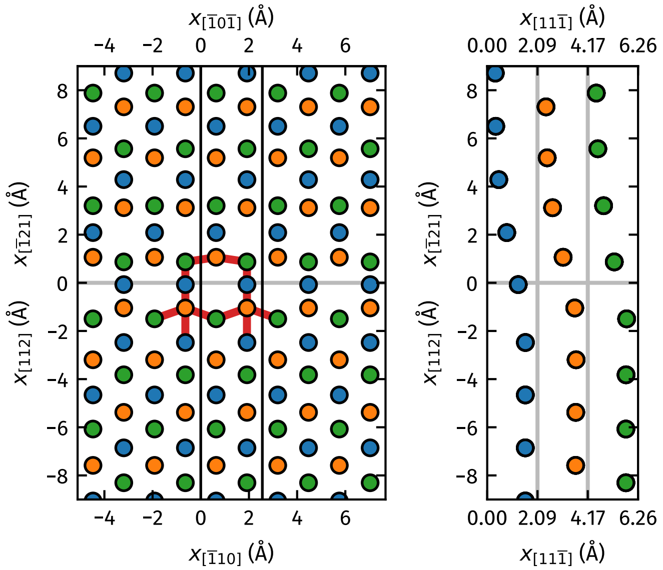


**Supplemental Fig. S16:** Zipper motifs in $\Sigma 3$ $[11\bar{1}]$ $\{112\}$ symmetric tilt GBs. Only one square is indicated, but the squares continue indefinitely along the GB in $\langle 011 \rangle$ direction without gaps. The motifs are thus equal to the previous zipper motifs minus the trapezoidal unit. The unit cell is marked by black vertical lines. A domino structure does not exist on the $\Sigma 3$ $[11\bar{1}]$ $\{011\}$ symmetric tilt GB.

## II. GRAIN BOUNDARY ENERGIES FOR Cu, Al, AND Ag

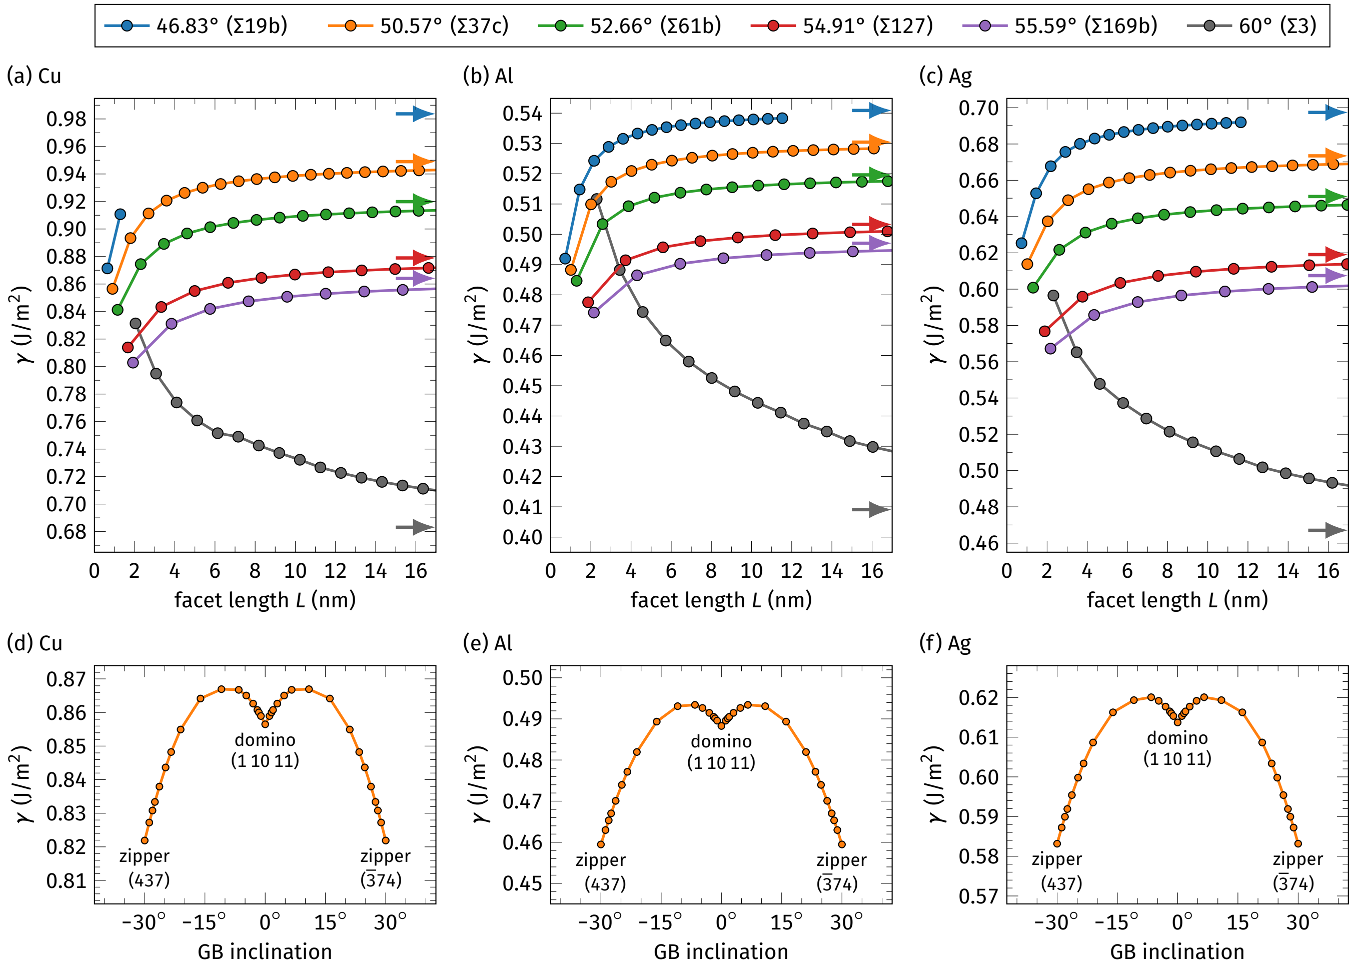


**Supplemental Fig. S17:** GB energies for Cu, Al, and Ag. (a)–(c) GB energies of GBs with an average plane corresponding to domino but different facet lengths. The arrows indicate the hypothetical energy of the faceted GBs if the junction did not contribute to the energy, i.e., $\gamma_{\text{zipper}}/\cos(30°)$. This also corresponds to the limit of infinite facet lengths. We can see that for $\theta < 60°$, the junctions have only an attractive interaction, thereby reducing the GB energy. The $\Sigma3$ GBs have a Burgers vector content in the junctions, ultimately leading to repulsion. (d)–(f) Energies for different inclination angles of the $\Sigma37$c GB (see also Fig. 8 in the main text).

## III. JUNCTION CHARACTERIZATION

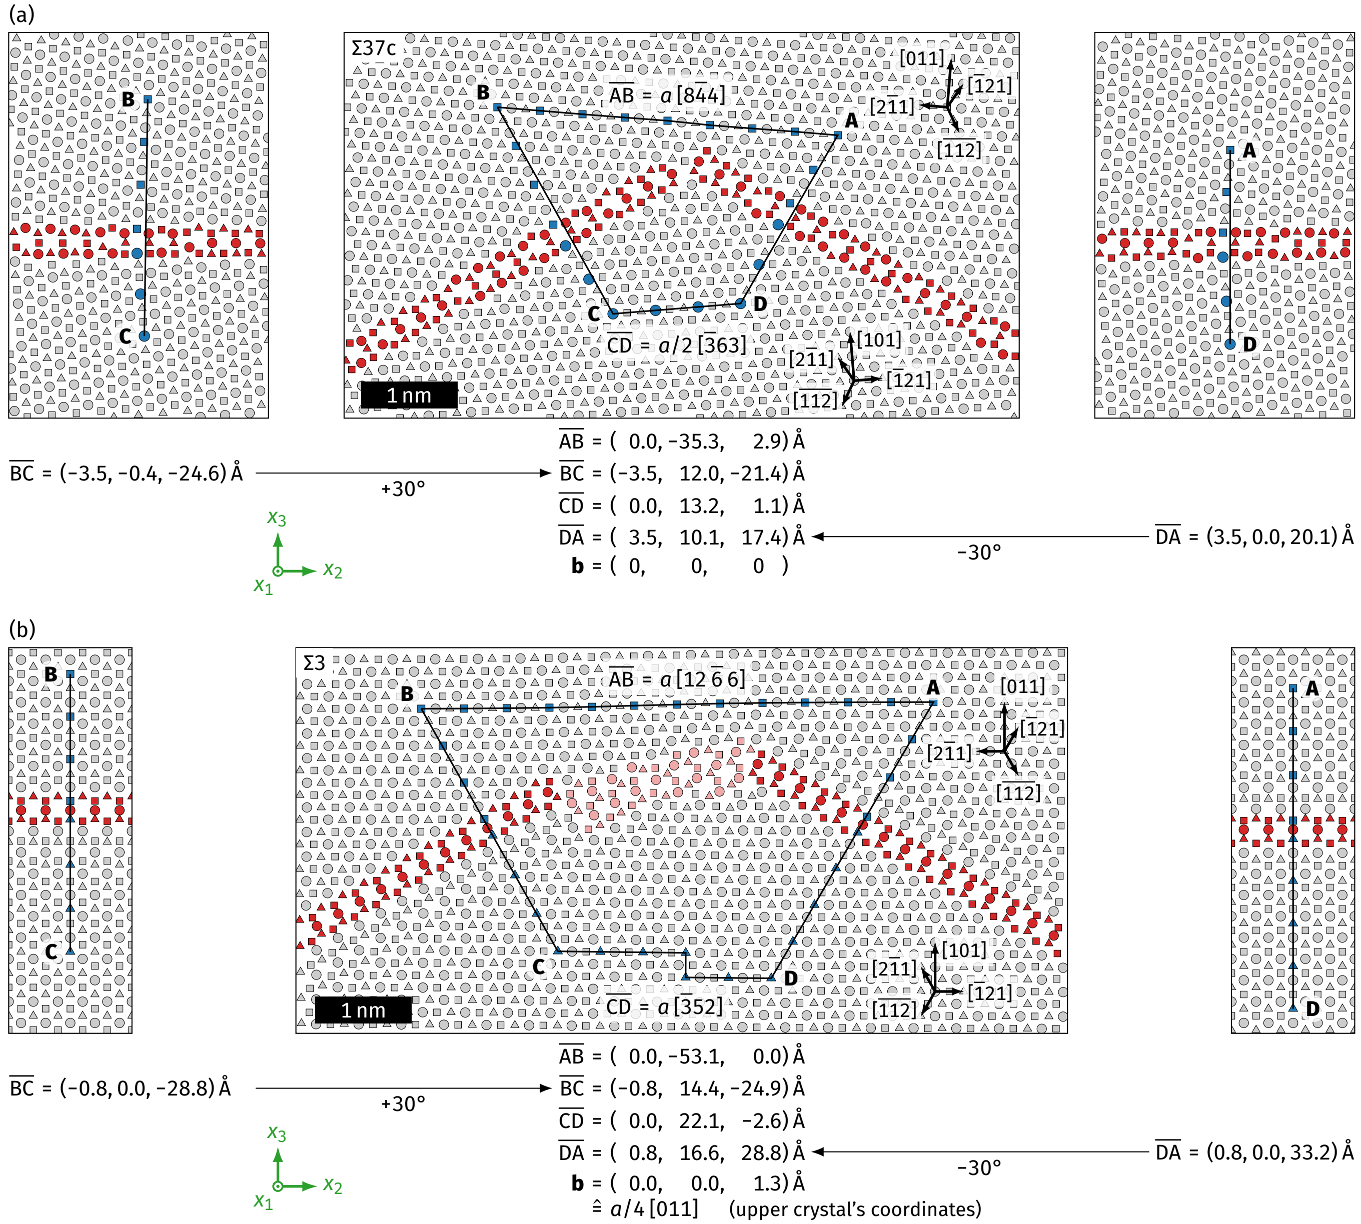


**Supplemental Fig. S18:** Burgers circuits around facet junctions in (a) Σ37c and (b) Σ3 GBs. These are the opposite junctions of the ones analyzed in Fig. 5 of the main text. See the Methods section and Fig. 5 in the main text for details on the construction of the circuits. We again obtain $\mathbf{b} = \mathbf{0}$ for the Σ37c GB. For Σ3, we obtain $\mathbf{b} = a/4[011]$ (coordinate system of the upper crystallite), which is—as expected—the opposite direction as the Burgers vector of the junction in Fig. 5(b) in the main text ($\mathbf{b} = a/4[0\bar{1}\bar{1}]$).

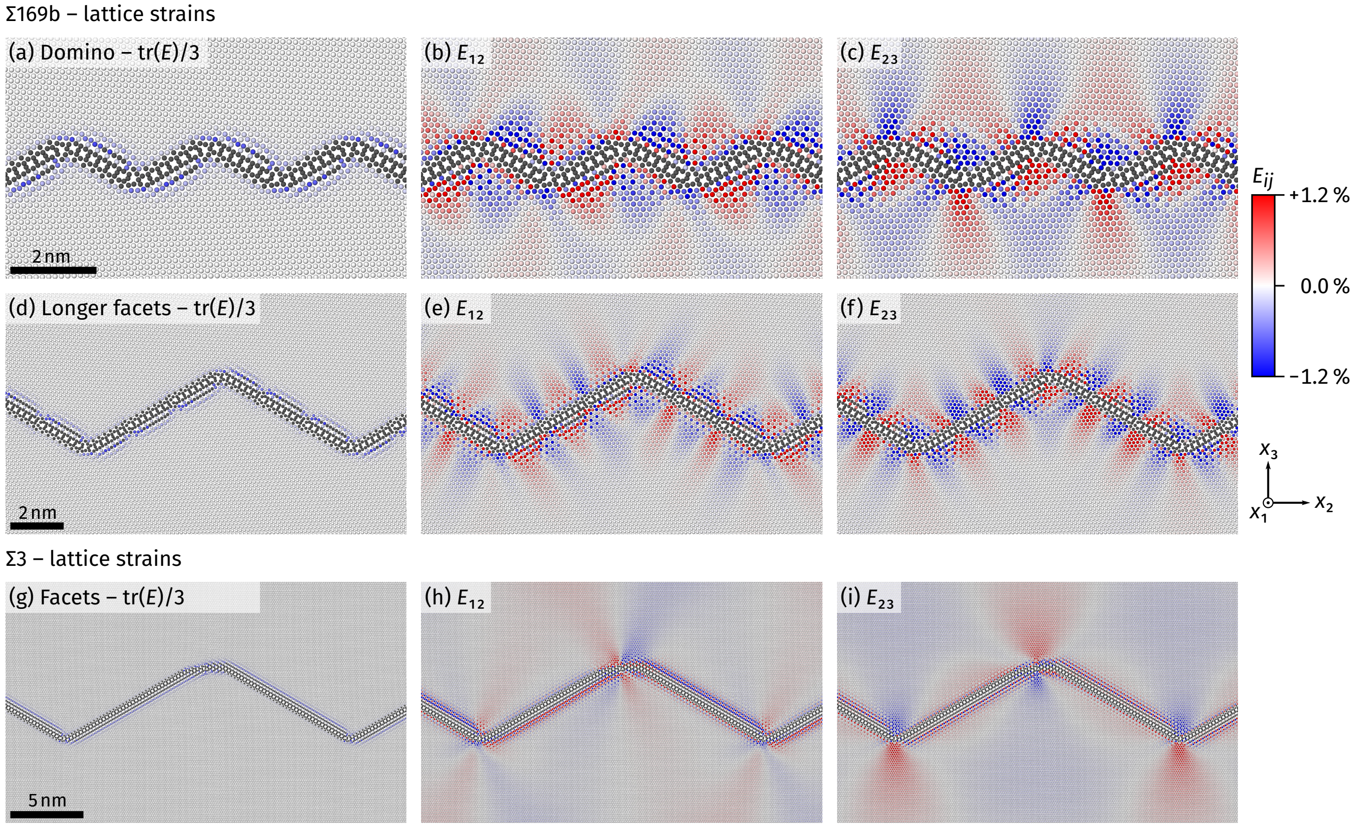


**Supplemental Fig. S19:** Lattice strains of Σ169b GBs (a–f) and a faceted Σ3 GB (g–i) obtained via polyhedral template matching [1] in OVITO [2]. This provides the strain of the individual atoms compared to their position in a perfect fcc lattice. Dark gray atoms are those that cannot be identified as belonging to elastically distorted fcc structures and for which strains cannot be calculated. Here, we report finite Green–Lagrangian strain tensors $E_{ij}$. We chose the Σ169b for visualization because the larger distance between the trapezoidal units makes the strain fields more easily visible. The first row shows the minimum facet length (i.e., the domino phase), while the second row shows a facet length with two intermediate trapezoidal units between the junctions. No long-ranged volumetric strains $\mathrm{tr}(E)/3$ occur. The alternating $E_{12}$ strains of the facets are compensated in domino, while they are more long-ranged in the longer facets. This compensation reduces the strain energy of the system. The $E_{23}$ components at the junctions are opposite, additionally highlighting the attractive line forces. The Σ3 GB, however, does not exhibit alternating, long-ranged strains $E_{12}$ that could lead to GB energy reduction, but the strain fields due to the Burgers vectors at the facet junctions are clearly visible. It must be noted again that the Burgers vectors at these junctions are opposite and therefore there is an attractive force between them; however, the total strain energy in the system is lower the fewer overall junctions exist, i.e., the longer the facets are. This is because each junction, even when partially compensated by an opposite Burgers vector, still contributes an additional positive strain energy.

## IV. EXCESS PROPERTIES

**Supplemental Table S-I:** Excess properties for Cu GBs that do not change when varying the inclination in 60° increments. Listed are the GB energy $\gamma$, the excess volume $[V]$, and the excess stresses $[\tau_{ii}]$ as defined in Ref. [3].

| | structure | $\gamma$ (J/m$^2$) | $[V]$ (Å) | $[\tau_{11}]$ (J/m$^2$) | $[\tau_{22}]$ (J/m$^2$) | GB plane | misorientation |
|---|---|---|---|---|---|---|---|
| Σ19b | domino | 0.871 | 0.220 | 0.29 | 0.24 | {178} | 46.83° |
| | zipper | 0.852 | 0.211 | 0.53 | −0.42 | {235} | |
| Σ37c | domino | 0.857 | 0.200 | −0.18 | 0.24 | {1 10 11} | 50.57° |
| | zipper | 0.822 | 0.189 | 0.19 | −0.37 | {347} | |
| Σ61b | domino | 0.841 | 0.184 | −0.49 | 0.18 | {1 13 14} | 52.66° |
| | zipper | 0.797 | 0.170 | −0.15 | −0.38 | {459} | |
| Σ127 | domino | 0.814 | 0.158 | −0.92 | 0.10 | {1 19 20} | 54.91° |
| | zipper | 0.761 | 0.144 | −0.59 | −0.40 | {6 7 13} | |
| Σ169b | domino | 0.803 | 0.147 | −1.09 | 0.07 | {1 22 23} | 55.59° |
| | zipper | 0.748 | 0.135 | −0.75 | −0.41 | {7 8 15} | |
| Σ3 | – | | | | | {011} | 60.00° |
| | zipper | 0.592 | 0.044 | −2.28 | −0.57 | {112} | |

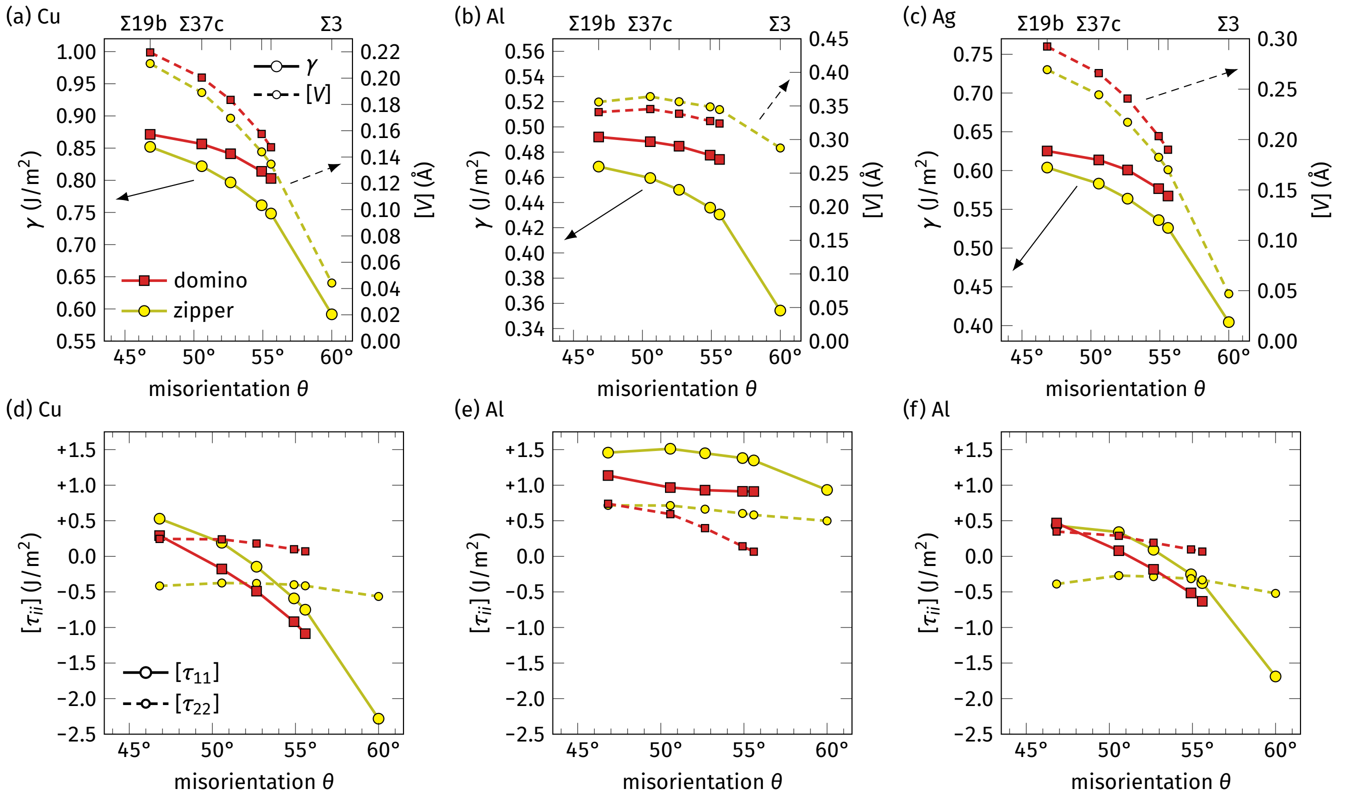


**Supplemental Fig. S20:** Graphical representation of Table S-I with additional data for Al and Ag. (a)–(c) Plots of GB energy as solid lines with scale on the left and excess volume as dashed lines with scale on the right. (d)–(e) GB excess stresses $[\tau_{11}]$ as solid lines and $[\tau_{22}]$ as dashed lines. Overall, higher misorientation angles $\theta$ lead to lower excess energies and volume, but no clear trend is observable for the excess stresses $[\tau_{ii}]$.

**Supplemental Table S-II:** Excess properties for Cu GBs that depend on the inclination. The vector [**B**] represents the microscopic translational degrees of freedom of the GB [3–5]. Notably, $[B_1]$ is the offset between $(11\bar{1})$ planes at the GB. The Σ GBs that are not shown and the results for Al and Ag are equivalent. Inclinations every 120° are crystallographically equivalent (3-fold symmetry along $[11\bar{1}]$) and thus have the same excess values. The domino always has the same sign of $[B_1]$ as the two zippers it is made of. While the zippers can have two degenerate states per inclination, combining for example the −30° and +30° zippers with positive $[B_1]$ would mean switching left and right zipper and lead to a different domino plane. Inclination is relative to the (arbitrary) domino we chose as reference. Planes are listed as top/bottom.

| | inclination | structure | $[B_1]$ (Å) | $[B_2]$ (Å) | $[B_3] - [V]$ (Å) | $[\tau_{12}]$ (J/m$^2$) | GB planes |
|---|---|---|---|---|---|---|---|
| Σ19b | −30° | **zipper** (right) | ±0.623 | ±0.607 | 0.293 | −0.19 | $(\bar{2}53)/(235)$ |
| | 0° | **domino** | −0.224 | 0.000 | 0.000 | 0.00 | $(178)/(718)$ |
| | 30° | **zipper** (left) | ±0.623 | ∓0.607 | 0.293 | +0.19 | $(325)/(5\bar{2}3)$ |
| | 60° | domino | +0.224 | 0.000 | 0.000 | 0.00 | $(8\bar{1}7)/(8\bar{7}1)$ |
| Σ37c | −30° | **zipper** (right) | ±0.713 | ∓0.256 | 0.210 | −0.15 | $(\bar{3}74)/(347)$ |
| | 0° | **domino** | −0.359 | 0.000 | 0.000 | 0.00 | $(1\,10\,11)/(10\,1\,11)$ |
| | 30° | **zipper** (left) | ±0.713 | ±0.256 | 0.210 | +0.15 | $(437)/(7\bar{3}4)$ |
| | 60° | domino | +0.359 | 0.000 | 0.000 | 0.00 | $(11\,\bar{1}\,10)/(11\,\overline{10}\,1)$ |
| | | | | ... | | | |
| Σ3 | −30° | zipper | ±0.85 | 0.00 | 0.738 | 0.00 | $(\bar{1}21)/(112)$ |
| | 30° | zipper | ±0.85 | 0.00 | 0.738 | 0.00 | $(112)/(2\bar{1}1)$ |

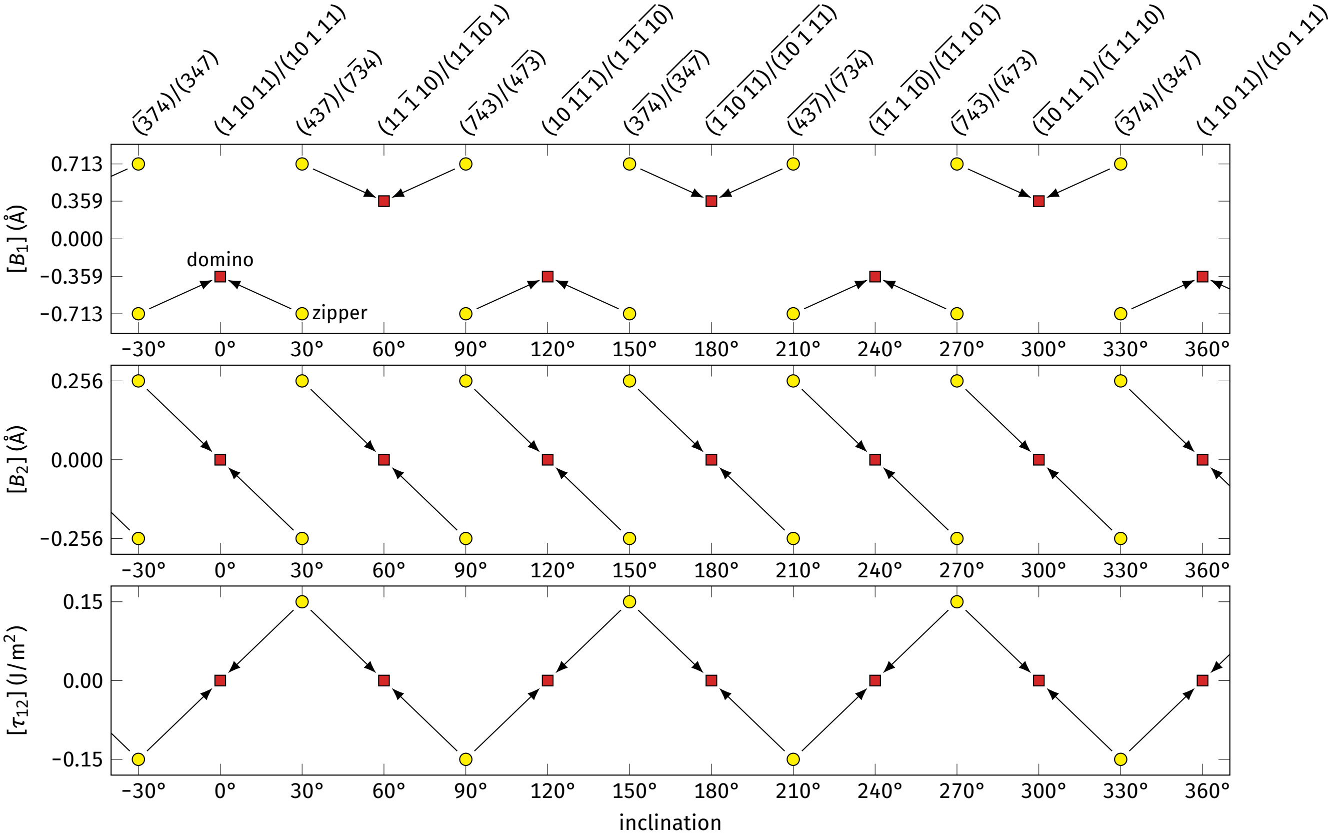


**Supplemental Fig. S21:** Graphical representation of Table S-II for Σ37c GBs in Cu. The arrows indicate which zipper structures combine into which domino structures.

## V. TRAPEZOIDAL UNIT AS VIRTUAL DISLOCATION

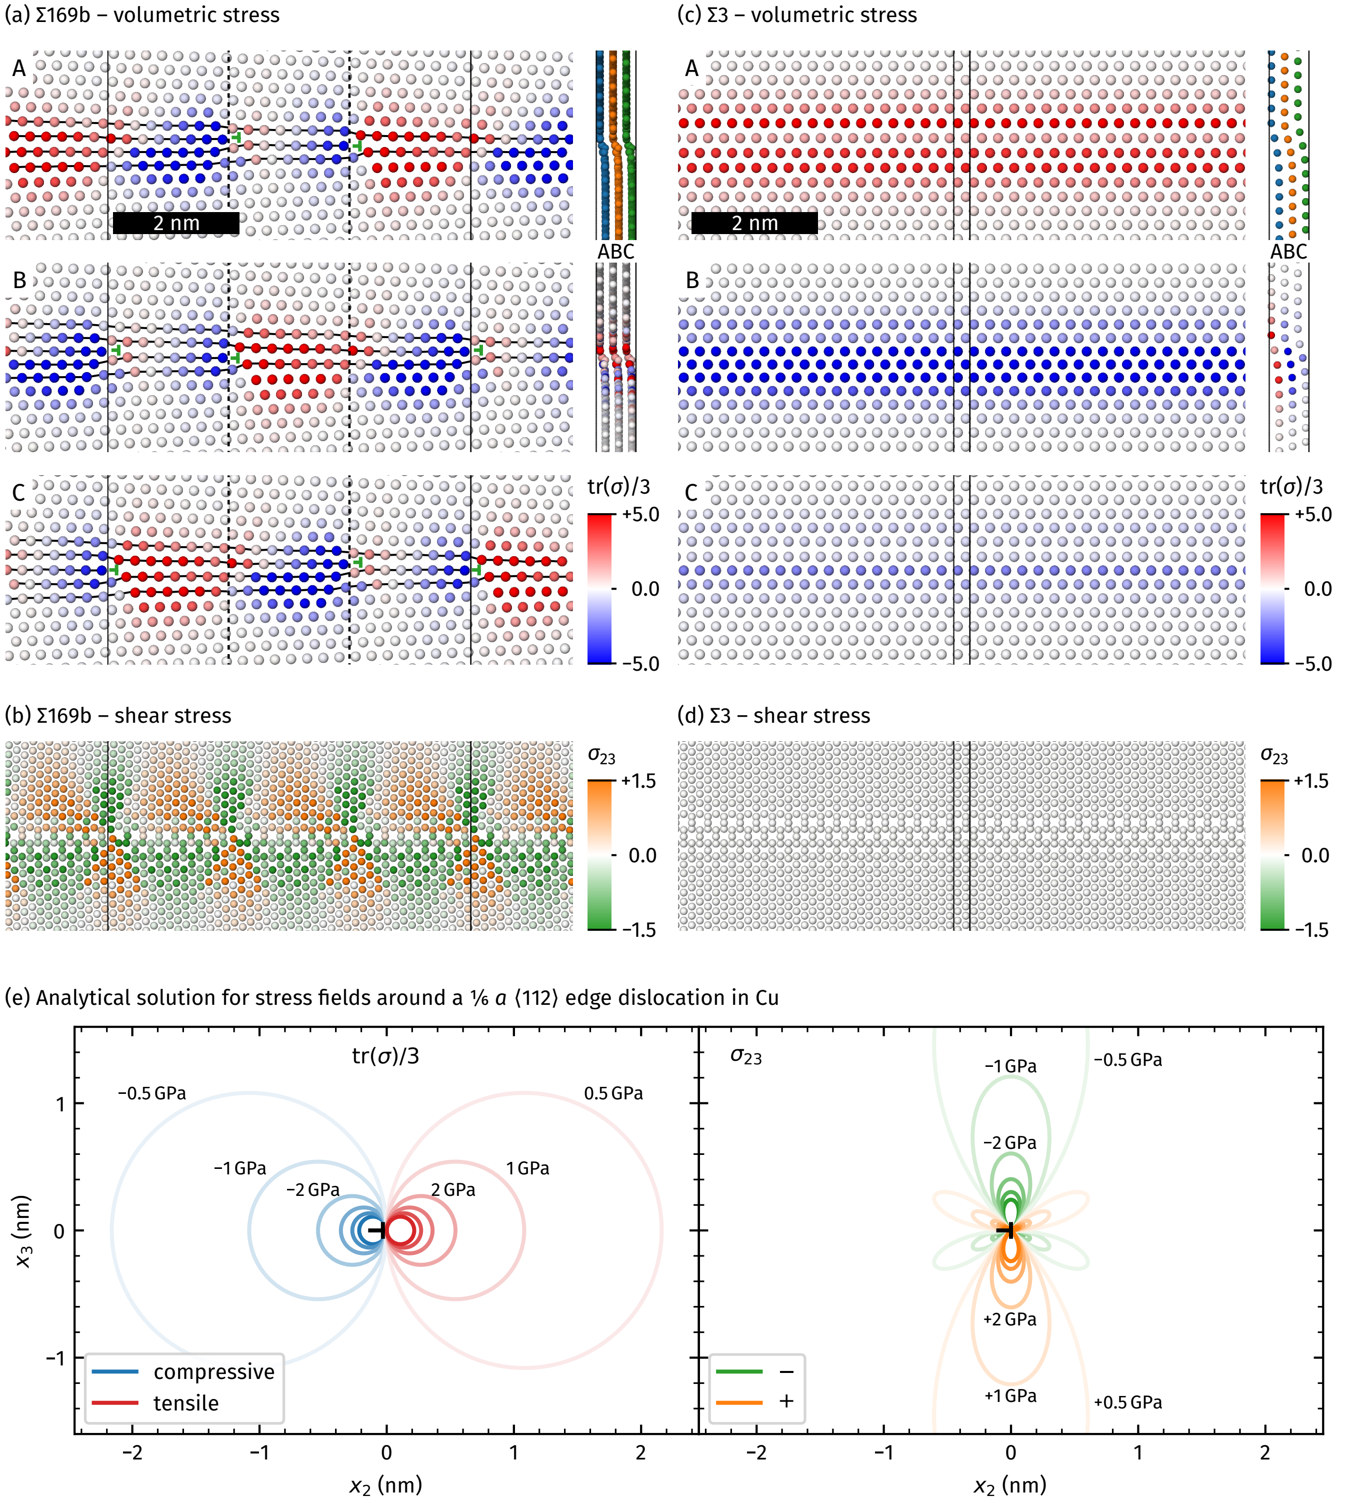


**Supplemental Fig. S22:** Stress fields in the (a)–(b) $\Sigma 169$b zipper structure and the (c)–(d) $\Sigma 3$ zipper structure. All stresses in GPa. The volumetric stresses (one third of the trace of the stress tensor) are plotted for each A, B, C $(11\bar{1})$ plane separately. This is because the stress field varies along the $[11\bar{1}]$ direction. In contrast to the $\Sigma 3$ GB, the $\Sigma 169$b GB exhibits 3 zipper motifs in its unit cell which are located on different $(11\bar{1})$ planes, leading to alternating stress states along horizontal direction (delimited by the dashed lines). Furthermore, additional stress fields resembling an edge dislocation are visible in the $\Sigma 169$b GB, cf. the plots in (e), which are analytical results for a $\mathbf{b} = a/6\langle 112\rangle$ edge dislocation [6].

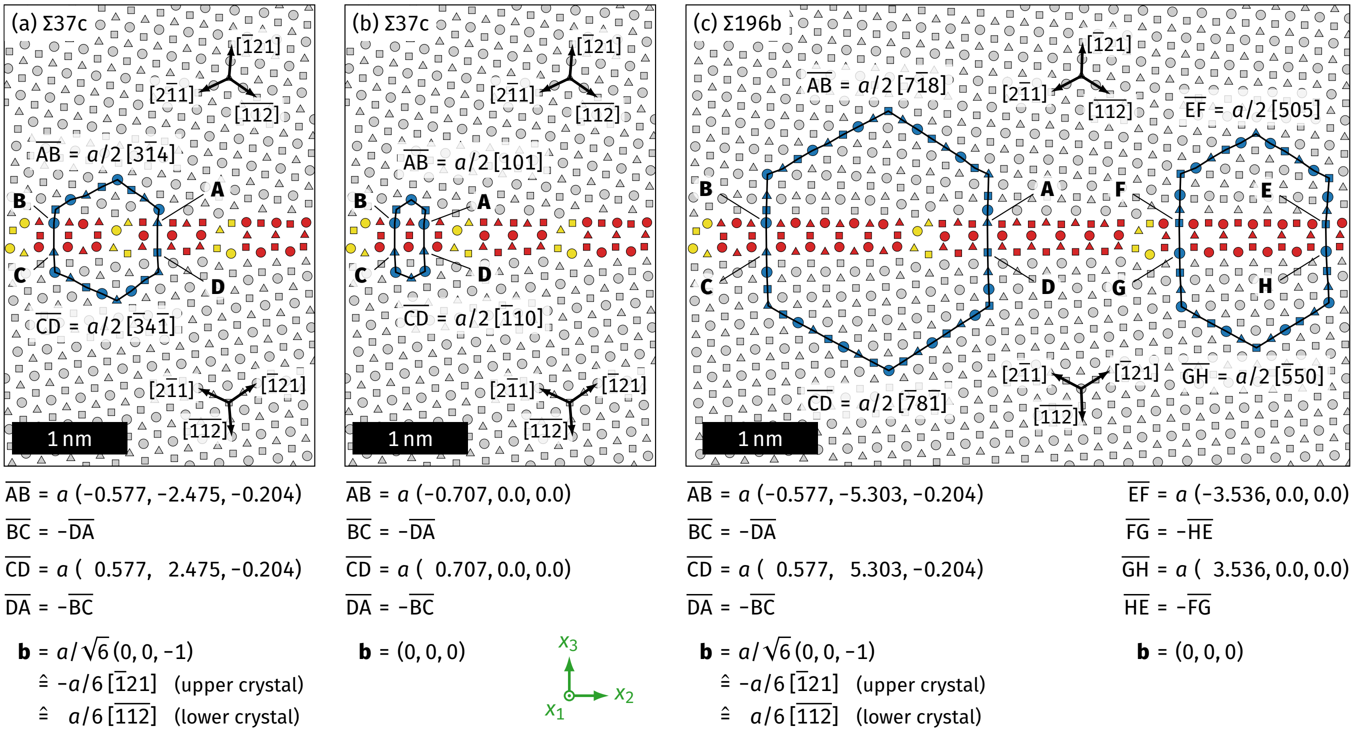


**Supplemental Fig. S23:** Burgers circuits to characterize the virtual dislocation in the zipper structure for $\theta < 60°$ in (a)–(b) Σ37c $[11\bar{1}]$ {347} and (c) Σ169b $[11\bar{1}]$ {8 7 15} GBs. Gray atoms are bulk atoms, while red atoms highlight the square GB motifs and yellow atoms highlight the trapezoidal unit. The shape of the symbols corresponds to the different $(11\bar{1})$ planes. Black lines and blue atoms represent the Burgers circuit.

We use a modified version of the method proposed by Medlin et al. [7], as also described in the Methods section of the main text. Here, two half-circuits are mapped in both crystallites, similar to a standard Burgers circuit in the bulk. We use the fact that the GB crossing (lines $\overline{BC}$ and $\overline{DA}$ in the figures) are at equivalent sites and cancel out. Therefore, we only need to convert the half-circuits into the same coordinate system. In the original method for tilt GBs, the coordinates of one half-circuit are rotated by the misorientation angle around the tilt axis and then both half-circuits are added together. This provides the dislocation content of GB defects compared to the pristine GB. In the present case we are interested in the dislocation content of the trapezoidal unit compared to the Σ3 GB ($\theta = 60°$). We thus rotate both the half-circuit $\overline{AB}$ and the half-circuit $\overline{CD}$ into the indicated image coordinate system $x_1$, $x_2$, $x_3$, *but using the rotation matrices that would apply to the 60° misorientation.* The resulting values are indicated below the figures.

Circuits around the trapezoidal unit in (a) and (c) on the left reveal a non-zero Burgers vector that is orthogonal to the GB plane. The corresponding dislocation line is along the $x_1$ direction (tilt axis), and we thus find $\mathbf{b} = a/6\langle 112\rangle$ type virtual edge dislocations compared to the pristine Σ3 GB. These virtual dislocations compensate the different misorientation, but should be called virtual dislocations because the absolute dislocation content of a Σ37c or Σ169b GB is lower than for a Σ3 GB. Due to the atomic arrangements (Fig. 2 in the main text) and the stress fields (Fig. S22), it nevertheless makes sense to treat the trapezoidal unit as an object with properties similar to an edge dislocation.

When the circuits do not include the trapezoidal unit and only go from red square to red square, as in (b) and left of (c), the resulting Burgers vector is zero. This makes sense, since the square units are the units of the Σ3 GB, which on their own lead to $\theta = 60°$.

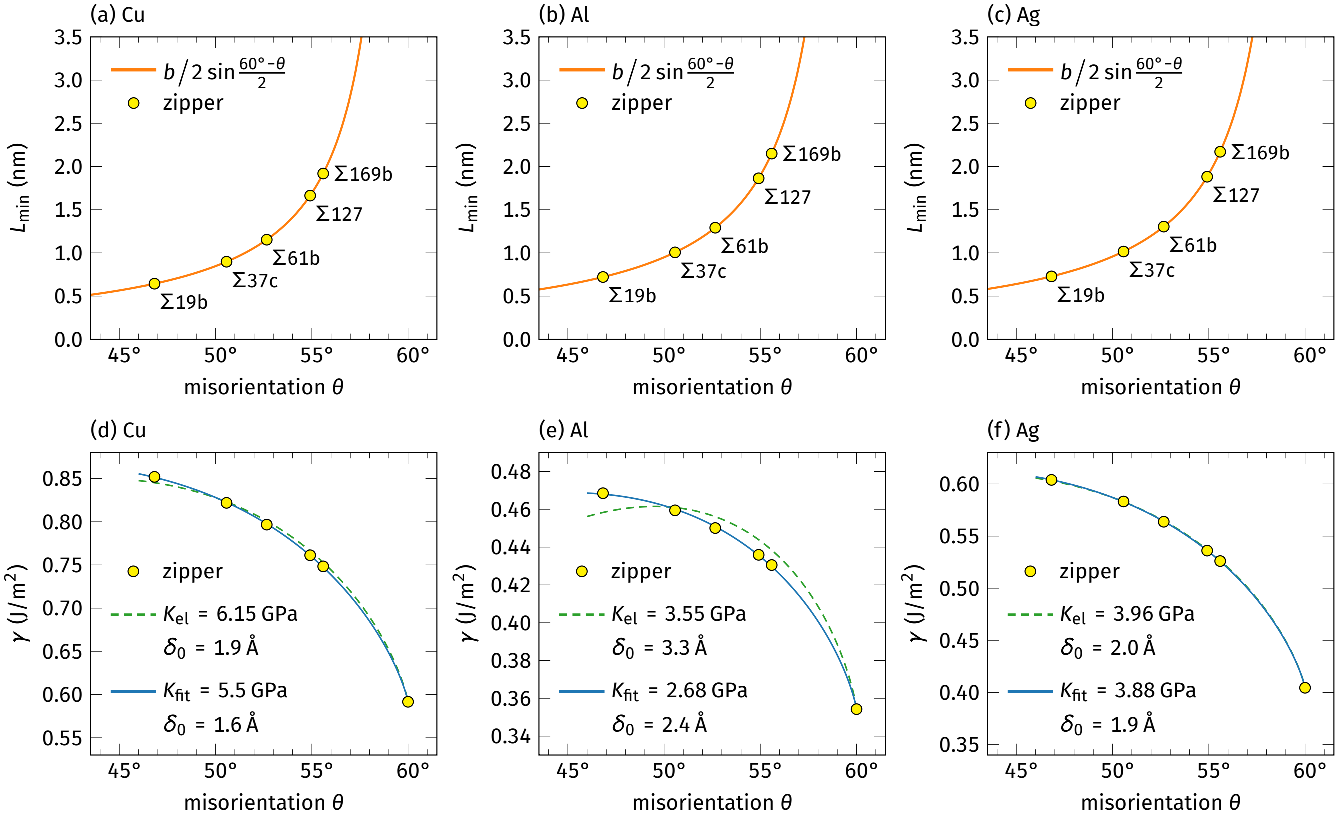


**Supplemental Fig. S24:** Energy of the zipper GBs. Extended data over Fig. 6 in the main text. If we treat the trapezoidal units as virtual edge dislocations, we can treat GBs with $\theta < 60°$ as a combination of a $\Sigma3$ GB and a low-angle GB with $\mathbf{b} = a/6\langle 112 \rangle$ dislocations. The energy of the zipper GB phase can be decomposed into

$$\gamma(\theta) = \gamma_{\Sigma3} + \frac{Kb^2}{L_{\min}(\theta)} \ln \frac{L_{\min}(\theta)}{\pi\delta_0},$$

where the second term is the energy of a low-angle GB [8, 9], defined by its dislocation interaction energy [8] with $K$ being an elastic constant [$= G/(4\pi - 4\pi\nu)$ for edge dislocations in isotropic materials with shear modulus $G$ and Poisson's ratio $\nu$] and $\delta_0$ an effective dislocation core size that also includes the core energy term [10, 11]. The length $L_{\min}$ represents the distance between trapezoidal units. Given that those are virtual $\mathbf{b} = a/6\langle 112 \rangle$ dislocations compared to $\Sigma3$, we can express

$$L_{\min}(\theta) = \frac{b}{2 \sin \frac{60° - \theta}{2}}$$

via a reversal of Read and Shockley's equation [12].

(a)–(c) The spacing $L_{\min}$ of the trapezoidal units corresponds to the prediction. (d)–(f) The energies were predicted in two different ways. First, we obtained $K = K_{el}$ from elasticity theory [13–16]. Since the parameter $\delta_0$ is purely empirical and also implicitly contains the dislocation core energy, it is always fitted. In a second step, we also used $K = K_{fit}$ as an empirical fit parameter. With the second approach we find a perfect match of the GB energies as a combination of $\gamma_{\Sigma3}$ and a low-angle GB energy. The value of $K_{el}$ is progressively worse from Ag to Cu to Al. This indicates that the stiffness of the GB itself likely plays a role, since the original formula was derived for bulk dislocations and pure low-angle GBs.

## SUPPLEMENTAL BIBLIOGRAPHY


[1] P. M. Larsen, S. Schmidt, and J. Schiøtz, Robust structural identification via polyhedral template matching, Modell. Simul. Mater. Sci. Eng. **24**, 055007 (2016).

[2] A. Stukowski, Visualization and analysis of atomistic simulation data with OVITO – the Open Visualization Tool, Modell. Simul. Mater. Sci. Eng. **18**, 015012 (2010), `https://ovito.org/`.

[3] T. Frolov and Y. Mishin, Thermodynamics of coherent interfaces under mechanical stresses. II. Application to atomistic simulation of grain boundaries, Phys. Rev. B **85**, 224107 (2012).

[4] T. Frolov and Y. Mishin, Thermodynamics of coherent interfaces under mechanical stresses. I. Theory, Phys. Rev. B **85**, 224106 (2012).

[5] T. Brink, L. Langenohl, H. Bishara, and G. Dehm, Universality of grain boundary phases in fcc metals: Case study on high-angle [111] symmetric tilt grain boundaries, Phys. Rev. B **107**, 054103 (2023).

[6] D. Hull and D. J. Bacon, *Introduction to Dislocations*, 5th ed. (Elsevier Butterworth–Heinemann, Oxford, UK, 2011).

[7] D. L. Medlin, K. Hattar, J. A. Zimmerman, F. Abdeljawad, and S. M. Foiles, Defect character at grain boundary facet junctions: Analysis of an asymmetric $\Sigma = 5$ grain boundary in Fe, Acta Mater. **124**, 383 (2017).

[8] F. R. N. Nabarro, Mathematical theory of stationary dislocations, Adv. Phys. **1**, 269 (1952).

[9] P. Lejček, *Grain Boundary Segregation in Metals* (Springer, Berlin, Germany, 2010).

[10] J. Han, S. L. Thomas, and D. J. Srolovitz, Grain-boundary kinetics: A unified approach, Prog. Mater Sci. **98**, 386 (2018).

[11] S. Pemma, R. Janisch, G. Dehm, and T. Brink, Effect of the atomic structure of complexions on the active disconnection mode during shear-coupled grain boundary motion, arXiv:2305.10275 [cond-mat.mtrl-sci] (2024).

[12] W. T. Read and W. Shockley, Dislocation models of crystal grain boundaries, Phys. Rev. **78**, 275 (1950).

[13] J. D. Eshelby, W. T. Read, and W. Shockley, Anisotropic elasticity with applications to dislocation theory, Acta Metall. **1**, 251 (1953).

[14] A. J. E. Foreman, Dislocation energies in anisotropic crystals, Acta Metall. **3**, 322 (1955).

[15] A. N. Stroh, Dislocations and cracks in anisotropic elasticity, Philos. Mag. A **3**, 625 (1958).

[16] J. P. Hirth and J. Lothe, *Theory of Dislocations*, 2nd ed. (Krieger Publishing Company, Malabar, Florida, USA, 1992).
